# Supplementary material for: Data-Augmented Counterfactual Learning for Bundle Recommendation
Source: arXiv:2210.10555 source file (2022-12-21)
Supplement: Supplementary file 1 [file 6.appendix.tex]

\section{Counterfactuals}
In the following we provide a background on Causal Inference that will form the basis for this paper.

\textbf{Definition 1} (Structural Causal Model (SCM)). A structural causal model ${M}$ consists of a set of independent (exogenous) random variables 
$ {u} = \{u_1,\dots,u_n\}$ with distribution $P({u})$,
a set of functions ${F} = \{f_1,\dots,f_n\}$, and a set of variables ${X} = \{X_1,\dots,X_n\}$ 

such that $X_i= f_i({P}{A}_i,{u}_i),\forall i$, 

where ${P}{A}_i  \subseteq  {X}\in X_i$is the subset of $X $ which are parents of $X_i$.
As a result, the prior distribution $P(u)$ and functions determine the distribution $P^{M}$.
An SCM defines the data generating process and the distribution of the observations. 
Using this model, we can investigate the consequences of intervention.

\textbf{Definition 2} (Interventional Distribution)

\textbf{Definition 5} (Backdoor Criterion)
A set of variables satisfies the backdoor criterion related to an ordered pair of variables

\textbf{Definition 3} (Intervention) [ 30,p.55] We distinguish between cases where a variable $X$ takes a value x naturally and cases where we fix $X=x$ by denoting the later $do(X=x)$. So $P(Y=y\mid X=x)$ is the probability that Y=y conditioned on finding $X=x$, while $P(Y=y\mid do(X=x))$ is the probability that $Y=y$ when we intervene to make $X=x$. Similarly, we write $P(Y=y\mid do(X=x),Z=z)$ to denote the conditional probability of $Y=y$, given $Z=z$, in the distribution created by the intervention $do(X=x)$.
To calculate the causal effect $P(y\mid do(x))$, the most fundamentalist approach is through causal graph manipulation. Technically, we remove all of $X $'s incoming edges from the original causal graph $\mathcal{G}$ to create the manipulated graph $\mathcal{G}_m$. And then we have have $P(y\mid do(x))=P_m(y\mid x)$, where $P_m$ is the manipulated probability. However, really implementing the manipulated causal graph $\mathcal{G}_m$ through direct intervention to calculate $P_m$ can be challenging or even impossible in practice. As a result, it would be nice if we can estimate $P(y\mid do(x))$ from purely observational data. The following causal effect rule answers this question.

\textbf{Definition 4} (The Causal Effect Rule) [30, p.59] Given a causal graph $G$ in which a set of variables $PA$ are designated as the parents of $X$, the causal effect of $X$ on $Y$ is given by:
\begin{equation}
\setlength{\abovedisplayskip}{3pt}
\setlength{\belowdisplayskip}{3pt}
\begin{aligned}
     P(Y=y\mid d o(X=x))&\ =\sum_{z} P(Y=y\mid X=x,PA=z)P(PA=z)\\&\ =\sum_{z}\frac{P(X=x,Y=y,PA=z)}{P(X=x\mid P A=z)}
\end{aligned}
\end{equation}
where $z$ ranges over all the combinations of values that the variables in $PA$ can take. The factor $P(X=x\mid PA=z)$ is the "propensity score".
The most important benefit brought by the above rule is that it enables us to calculate the causal effect between two variables based on passive observational data — we see that the right side of the equation does not include do-calculations any more. However, enumerating all parents' value combinations is still rather complicated. The following backdoor criterion solves the problem.

\textbf{Definition 5} (Backdoor Criterion) [30, p.61] A set of variables $Z$ satisfies the backdoor criterion related to an ordered pair of variables $(X,Y)$ in a causal graph $\mathcal{G}$ if $Z$ satisfies both (1) No node in $Z$ is a descendant of $X$ and (2) $Z$ blocks every path between $X$ and $Y$ that contains an arrow into $X$.
If a set of variables $Z$ satisfies the backdoor criterion for $X$ and $Y$, then the causal effect of $X$ on $Y$ is given by the formula:
\begin{equation}
\setlength{\abovedisplayskip}{3pt}
\setlength{\belowdisplayskip}{3pt}
\begin{aligned}
P(Y=y\mid do(X=x))=\sum_{z} P(Y=y\mid X=x,Z=z)P(Z=z)
\end{aligned}
\end{equation}
through which we can also estimate $P(y\mid do(x))$ from observational data but it may only need much fewer variables.
The backdoor criterion can be generalized to z-specific causal effect $P(Y=y\mid do(X=x),Z=z)$, in which we care about the causal effect of $X$ on $Y$ under a specific value $Z=z$[30,p.70]. 
If we can find a set of variables $S$ such that $S\cup Z$ satisfies the backdoor criterion ( $S$ may include $Z$ ), then the z-specific causal effect can be estimated from observational data:
\begin{equation}
\setlength{\abovedisplayskip}{3pt}
\setlength{\belowdisplayskip}{3pt}
\begin{aligned}
&P(Y=y\mid d o(X=x),Z=z)\\=&\ \sum_{s} P(Y=y\mid X=x,S=s,Z=z)P(S=s\mid Z=z)
\end{aligned}
\end{equation}
where the summation goes over all value combinations of $S$.
Finally, counterfactual analysis aims to answer queries that go beyond the observational data. 
In notation, we use $Y_{X=x}(U=u)=y$, or simplified as $Y_x(u)=y$, to represent the counterfactual sentence " $Y$ would be $y$ had $X$ been $x$, in situation $U=u$ ", though the observed value of $X$ in real world is not $x$. The mathematical definition of counterfactual is as follows.

\textbf{DEFINITION 6} (Counterfactual) [30, p.94] Let $M$ be the original structural causal model, and $M_x$ be the modified version of $M$ with the equation of $X$ replaced by $X=x$. 
Then the formal definition of the counterfactual $Y_x(u)$ is $Y_x(u)=Y_{M_x}(u)$, i.e., the counterfactual $Y_x(u)$ in model $M$ is defined as the solution for $Y$ in the "surgically modified" submodel $M_x$.
Further more, we use $P\left(Y_x=y\right)$ to represent the probability of $Y=y$ had $X$ been $x$, and use $E\left[Y_x\right]$ to represent the expected value of $Y$ had $X$ been $x$.

\section{Part B}
